# Supplementary material for: CustomSketching: Sketch Concept Extraction for Sketch-based Image Synthesis and Editing
Source: arXiv:2402.17624 source file (2024-02-27)
Supplement: Supplementary file 1 [file limitation.tex]

\begin{figure}[t]
    \centering
    \includegraphics[width=\linewidth]{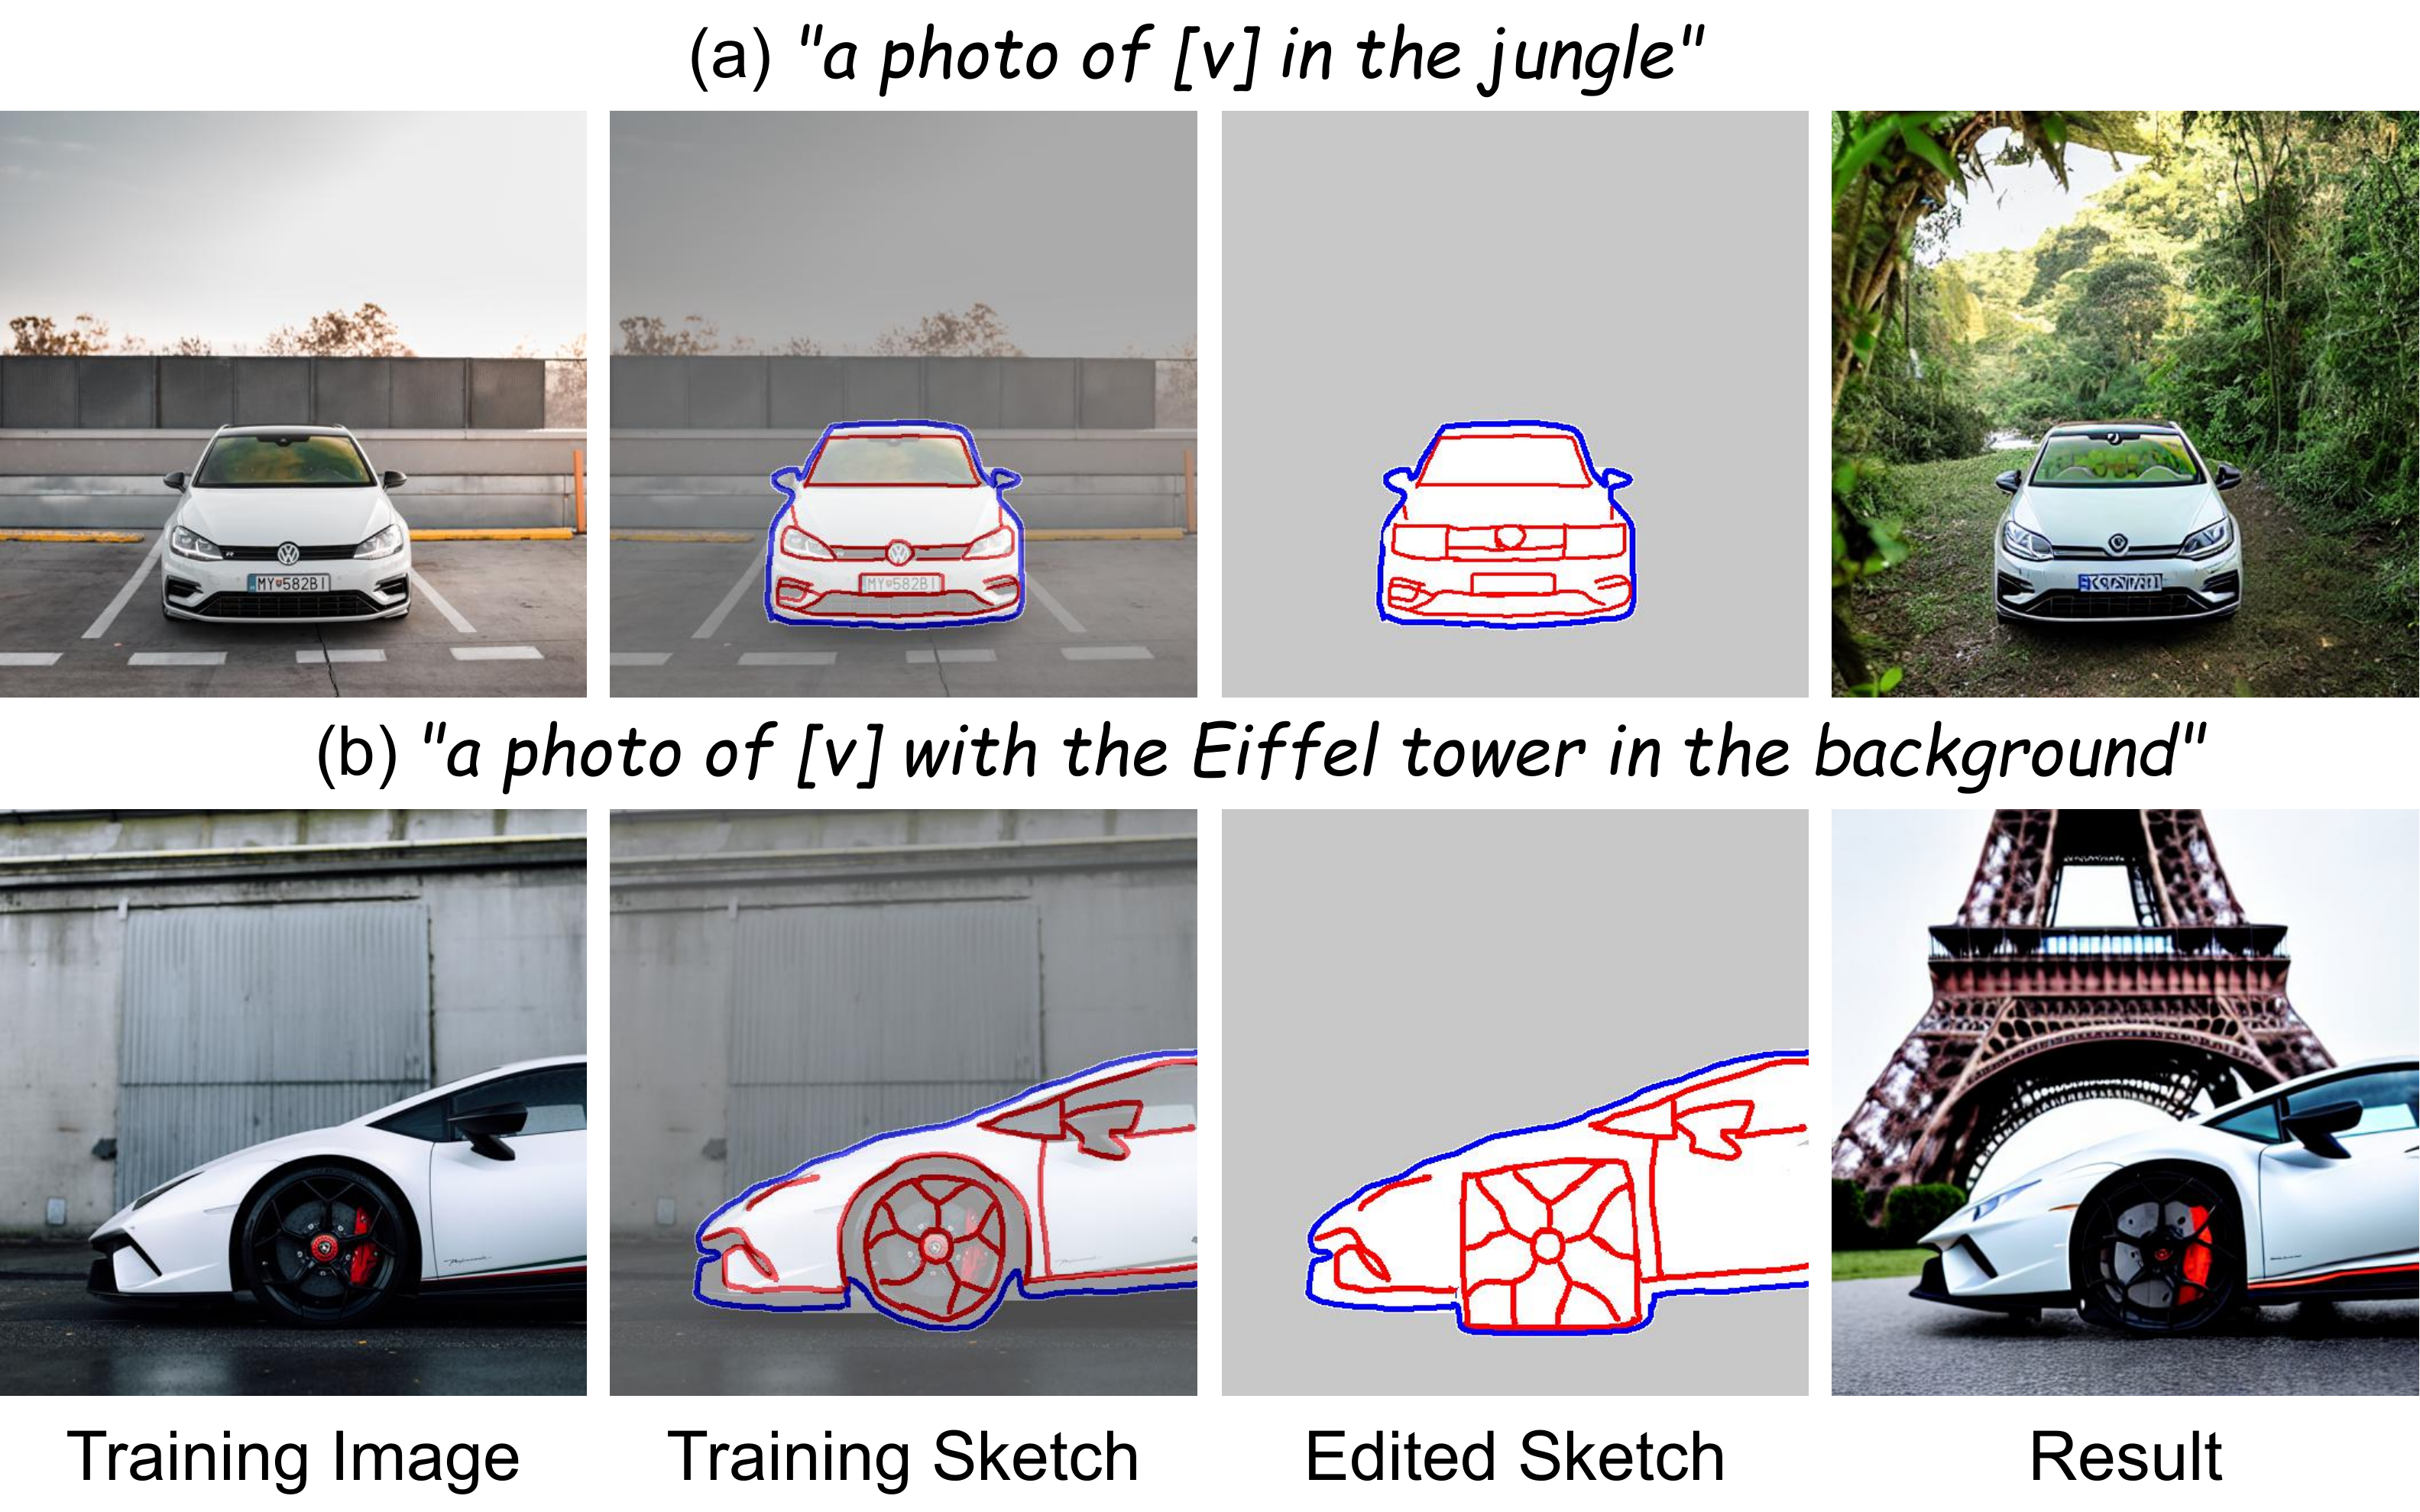}
    \caption{
    {Two failure cases {of} %generated by 
    our method. (a) Our method could not change the car's tiny details by sketching thin strokes. (b) Our method struggles to generate a rectangular car tier, which is against the prior of the pre-trained model. 
    }}
    \label{fig:limitation}
\end{figure}
